# Supplementary material for: Splat-Nav: Safe Real-Time Robot Navigation in Gaussian Splatting Maps
Source: arXiv:2403.02751 source file (2025-01-11)
Supplement: Supplementary file 1 [file appendix_v0.tex]

% \section*{Appendix}
% \label{sec:appendix}
\appendices

\section{Proof of Proposition~\ref{prop:ellipsoidtest2}}
\label{app:prop_gen_eigen_proof}
This proposition was stated by \cite{alger2020ellipsoidtest} without proof. We provide the proof here. The goal is to diagonalize both $\Sigma_a$ and $\Sigma_b$ in such a way that they share the same eigenbasis. In this way, the matrix inversion amounts to a reciprocal of the eigenvalues. We can find such an eigenbasis through the generalized eigenvalue problem, which solves the following system of equations ${\Sigma_a\phi_i = \lambda_i \Sigma_b \phi_i.}$
    % \begin{equation*}
    %     \Sigma_a\phi_i = \lambda_i \Sigma_b \phi_i.
    % \end{equation*}
    These generalized eigenvalues and eigenvectors satisfy the identity ${\Sigma_a \phi = \Sigma_b \phi \Lambda.}$
    % \begin{equation*}
    %     \Sigma_a \phi = \Sigma_b \phi \Lambda.
    % \end{equation*}
    
    To solve the generalized eigenvalue problem, we utilize the fact that $\Sigma_a$ and $\Sigma_b$ are symmetric, positive-definite, so the Cholesky decomposition of $\Sigma_b = L L^T$,
    where $L$ is lower triangular. This also means that we can represent $\Sigma_a$ by construction as
    \begin{equation*}
        \Sigma_a = L C L^T = L V \Lambda V^T L^T,
    \end{equation*}
    where $C$ is also symmetric, positive-definite, so its eigen-decomposition is $C = V \Lambda V^T$, where the eigenvectors $V$ are orthonormal $V^T V = I$. To retrieve the original eigenbasis $\phi$, we solve the triangular system $L^T \phi = V$. A consequence of this solution is that 
    \begin{equation*}
    V^T V = \phi^T L L^T \phi = \phi^T \Sigma_b \phi = I.
    \end{equation*}
    Moreover, this means that $\Sigma_b = \phi^{-T} \phi^{-1}$. We can show that $\Lambda$ and $\phi$ indeed solve the generalized eigenvalue problem through the following substitution
    \begin{equation*}
        \Sigma_a \phi = LV\Lambda V^T L^T \phi = \underbrace{L L^T}_{\Sigma_b} \phi \Lambda \phi^T \underbrace{L L^T}_{\Sigma_b} \phi = \Sigma_b \phi \Lambda \underbrace{\phi^T \Sigma_b \phi}_{I},
    \end{equation*}
    where $\Lambda = \diag (\lambda_i)$ is the diagonal matrix of eigenvalues.
    
    As a result, we can write the matrix inversion in Theorem \ref{thm:ellipsoidtest1} as the following
    \begin{equation*}
    \begin{split}
        \left[ \frac{1}{1-s}\Sigma_a + \frac{1}{s}\Sigma_b \right] ^{-1} &= 
        \left[\frac{1}{1-s} \Sigma_b \phi \Lambda \phi^T \Sigma_b  + \frac{1}{s} \Sigma_b \right]^{-1} \\ 
        &= \left[\phi^{-T} \left(\frac{1}{1-s} \Lambda + \frac{1}{s} I \right) \phi^{-1} \right]^{-1} \\
        &= \phi\left[\frac{1}{1-s} \Lambda + \frac{1}{s} I \right]^{-1} \phi^T \\
        &= \phi \; \diag\left(\frac{s(1-s)}{1 + s(\lambda_i - 1)} \right) \; \phi^T.
    \end{split}
    \end{equation*}
    Multiplying the left and right by $\mu_b - \mu_a$ completes the proof.

\section{Proof of Corollary~\ref{cor:intersection_test_sampling}}
\label{app:proof_intersection_test_sampling}
Using a finite number of samples, the test can fail (no sample points yield $K(s) > 1$) or succeed (there is a sample point such that $K(s) > 1$). Should the test succeed, by definition, there is no intersection. If it fails, there either exists an un-sampled point with $K(s) > 1$ or such a point does not exist. If no such point exists, then the test remains correct in predicting collision. If such a point exists, it simply means our test predicted collision while in reality the ellipsoids are intersection-free. In other words, using finite samples leads to a safe, but conservative test. Due to the concavity of $K(s)$, more samples will asymptotically decrease the conservativeness. 

\section{Proof of Proposition~\ref{prop:supp_hyperplane}}
\label{app:proof_supp_hyperplane}
From Proposition~\ref{prop:ellipsoidtest2}, we know that we must find an $x$ such that $K(s) > 1$ for all ellipsoids in the test set $\mathcal{G}^*$.
We will approximate this safe set as a polytope.
Given a test point $x^*$ and the $j$th ellipsoid in the collision test set $\mathcal{G}^*$, we can use our collision test (Corollary \ref{cor:gs_intersection_test}) to derive these polytopes. Notice in \eqref{eq:gs_ellipsoid_test} that $\mu_a$ represents the position of the robot (i.e., the test point $x^*$) and $\mu_b$ is the centroid of ellipsoid $j$. Once we find the value $s^*$ that maximizes $K(s)$, the safety test is a quadratic constraint of the test point $x^*$, namely $\Delta_j^T Q_j \Delta_j > 1$.

To derive the supporting hyperplane for the safety check, we will first find the point on the ellipsoid and then linearize our test about this point.
Let $f_j(x) = (x-\mu_j)^T Q_j (x-\mu_j)$. Note that $f_j(x^*) = \Delta^T_j Q_j \Delta_j = (k_j^*)^2$.
We can immediately see that point $x_0 = \mu_j + \frac{1 + \epsilon}{k_j^*} \Delta_j$ will be outside of the ellipsoid for any $\epsilon > 0$ since $f_j(x_0) = (x_0-\mu_j)^T_j Q_j (x_0-\mu_j) = \frac{(1+\epsilon)^2}{(k_j^*)^2} \Delta_j^T Q_j \Delta_j = (1 + \epsilon)^2 > 1$. Note that this point $x_0$ lies on the ray starting from the center of the ellipsoid $\mu_j$ and passing through the center of the robot at $x^*$.
We then linearize the constraint $f_j(x)$ about $x_0$. 
Taking the derivative yields $\frac{df_j}{dx}(x) = 2 (x-\mu_j)^T Q_j$.
The linear approximation of the constraint is then $f_j(x) \approx f_j(x_0) + \left[\frac{df_j}{dx}(x_0)\right] (x - x_0) = (1+\epsilon)^2 + 2 (x_0-\mu_j)^T Q_j (x - x_0) \geq 1$.
Plugging in $x_0 = \mu_j + \frac{1+\epsilon}{k_j^*}\Delta_j$ and simplifying yields the given expression $\Delta^T_j Q_j x \geq \frac{k_j^*}{1+\epsilon} + \Delta^T_j Q_j \mu_j$.

We need to also prove that the above constraint is a supporting hyperplane by showing that all feasible points when the constraint is equality is necessarily outside of the ellipsoid parametrized by $Q_j$. Recall that $x_0 = \mu_j + \frac{\Delta_j}{k_j^*}$ is a point both on the surface of the ellipsoid and on the hyperplane. Therefore, all feasible points on the hyperplane can be expressed as $x = x_0 + \delta$, where $\Delta_j^T Q_j \delta = 0$. If the hyperplane supports the ellipsoid parametrized by $Q_j$, then necessarily $f(x) = (x-\mu_j)^T Q_j (x-\mu_j) \geq 1$. For all points on the hyperplane, the ellipsoid constraint evaluates to 
\begin{multline*}
% \begin{split}
    f_j(x_0 + \delta) = \left(\frac{1+\epsilon}{k_j^*}\Delta_j + \delta\right)^T Q_j \left(\frac{1+\epsilon}{k_j^*}\Delta_j + \delta \right) \\
    =\underbrace{\frac{(1+\epsilon)^2}{(k_j^*)^2}\Delta_j^T Q_j \Delta_j }_{ = (1+\epsilon)^2}+ \underbrace{\delta^T Q_j \delta}_{\geq 0} + \underbrace{\frac{2(1+\epsilon)}{k_j^*}\Delta_j^T Q_j \delta}_{= 0} > 1.
% \end{split}
\end{multline*}
Therefore, the constraint in Proposition \ref{prop:supp_hyperplane} is a supporting hyperplane.

\section{Planning Computation Times}
In addition to outperforming other existing methods in safety and path length of computed paths (Fig. \ref{fig:planning_quantitative},\ref{fig:ablation}), our Splat-Plan method achieves faster computation times compared to the point-based motion planners RRT* and NeRF-Nav; generates smooth trajectories unlike the RRT*, NeRF-Nav, and A*; and detects infeasible planning problems.
We remind the reader of the following baselines: RRT*, A*, and polytopic A*. RRT* (implemented in OMPL) replaces the default collision checker with our ellipsoid-to-ellipsoid collision test in Proposition 1. The A* methods use the means of the Gaussians in GSplat to create a binary occupancy grid. A* simply plans a shortest path through the binary grid. Polytopic A* goes one step further, constructing safe polytopes through Proposition \ref{prop:supp_hyperplane} on the A* waypoints, from which it computes a B-spline trajectory passing through all the polytopes. Splat-Plan is a further refinement of the Polytopic A* algorithm. Instead of a single instance of A*, we iterate between querying A* and updating the binary occupancy grid at the A* waypoints that are unsafe via the collision test in Proposition \ref{prop:ellipsoidtest2}. Typically, the Splat-Plan method requires only a handful of A* iterations (${< 5}$), and the generation of polytopes for approximately $100$ A* waypoints runs at approximately $100$ Hz.

Splat-Plan is much faster than RRT* and NeRF-Nav \cite{adamkiewicz2022vision} due to our method's inherent sampling efficiency, as noted in Table~\ref{tab:planning_times}. The faster computation time in Splat-Plan results primarily from the fast safe polytope generation procedure. Because both of these baselines also test/measure safety point-wise, they have finite resolution. Therefore, these baselines may not dynamically feasible for some robotic tasks, and may be unsafe in certain regions of the computed trajectory, if the resolution is insufficient. 

The creation of polytopes also endows our method with the ability to fail gracefully. A smooth curve can be created from the start to goal locations so long as a connected series of safe polytopes are given. Since the polytopes generated are inherently safe, we can simply check for overlap between consecutive pairs of polytopes. In this work, for simplicity, we choose to solve an LP to determine overlap. Typically, this operation can be performed at more than 10 Hz for the entire trajectory. Of course, less computationally-intensive methods exist, such as the GJK algorithm to determine collision between convex objects. Using the connectivity of polytopes as a failure signal, we observe that by not updating the occupancy grid and subsequently executing A*, polytopic A* can only achieve feasible safe trajectories $55\%$ out of $100$ configurations. This is due to the corner phenomenon in Remark \ref{remark:connectivity}, where safe polytopes existing on both sides of an ellipsoidal wall are disconnected.

Since Splat-Plan requires the use of A* to initialize a path to generate the safety polytope corridors, it will necessarily be slower than these A* baselines. However, we note that in the Full Trajectory regime, the dominating cost is the calculation of the B-spline due to the number of polytopes in the constraints, with many facets per polytope. This QP was solved using CVXPY with the Clarabel solver. We note that the computation time associated with the B-spline computation procedure can be reduced using embedded solvers or faster programming languages.

\begin{table}[th]
	\centering
	\caption{Comparison of Full Trajectory planning algorithm computation times.}
	\label{tab:planning_times}
	\begin{adjustbox}{width=\linewidth}
		{\begin{tabular}{l c c c}
				\toprule
    
				Algorithm & Times (s) & Smooth & Failure Signal\\
				\midrule
    
				NeRF-Nav \cite{adamkiewicz2022vision} & $2.33$ & $\times$ & $\times$\\
    
				RRT* & $9.49 \pm 5.13$ & $\times$ & $\times$\\
    
				A* & $0.051 \pm 0.0096$ & $\times$ & $\times$\\

				Non-iterative, Polytopic A*& $0.13 \pm 0.037$ & \checkmark & \checkmark (55$\%$)\\
    
				Splat-Plan (\textbf{ours}) & $0.90 \pm 0.29$ & \checkmark & \checkmark (100$\%$)\\
				\bottomrule    
		\end{tabular}}
	\end{adjustbox}
\end{table}

% \begin{table}[th]
% 	\centering
% 	\caption{Comparison of Full Trajectory planning algorithm computation times.}
% 	\label{tab:planning_times}
% 	\begin{adjustbox}{width=\linewidth}
% 		{\begin{tabular}{l c c c}
% 				\toprule
    
% 				Algorithm & Times (s) & Smooth & Failure Signal\\
% 				\midrule
    
% 				NeRF-Nav \cite{adamkiewicz2022vision} & $2.325$ & $\times$ & $\times$\\
    
% 				RRT* & $9.489 \pm 5.128$ & $\times$ & $\times$\\
    
% 				A* & $0.0508 \pm 0.00956$ & $\times$ & $\times$\\

% 				Non-iterative, Polytopic A*& $0.1222 \pm 0.03636$ & \checkmark & \checkmark (55$\%$)\\
    
% 				Splat-Plan (\textbf{ours}) & $0.892 \pm 0.2896$ & \checkmark & \checkmark (100$\%$)\\
% 				\bottomrule    
% 		\end{tabular}}
% 	\end{adjustbox}
% \end{table}

Since the polytope and A* computation procedures are relatively fast, while computation of the B-spline is relatively slow, we can compute the B-spline for some small time step in the future, in a receding-horizon manner. In our experiments, this amounted to fitting a B-spline through the current and next polytope. Since the Full Trajectory method finds a connected series of polytopes and is therefore always able to fit a B-spline connecting the start position to goal position, the Local Trajectory method can also still guarantee safety and feasibility since the entire constraint set is separable based on time, at the expense of the optimality of the solution. 

We found the 55$\%$ success rate of the polytopic A* to be surprisingly high, which speaks to the ability of our polytopes to be generated even when query points are unsafe. To push the limits of generalizability of the polytopes, we implemented a simple line following planner based on the polytopes. Specifically, in this baseline, we query a polytope at the robot's current position, and another polytope at a point some small distance away ($0.02$ in our evaluations) on the line between the current position and the goal position, then solve for a B-spline. Such a method did not yield connected polytopes for $18\%$ of configurations, and got stuck (ran for over $200$ iterations) for $24\%$ of configurations. Note that while the robot was stuck, the B-spline was still guaranteed safe (Fig. \ref{fig:ablation}).

\begin{table}[th]
	\centering
	\caption{Comparison of Local Trajectory planning algorithm computation times.}
	\label{tab:ablation_times}
	\begin{adjustbox}{width=\linewidth}
		{\begin{tabular}{l c c c}
				\toprule
    
				Algorithm & Times (s) & Smooth & Failure Signal\\
				\midrule
    
				Line Following & $0.015 \pm 0.0086$ & \checkmark & \checkmark (58$\%$)\\
    
				Splat-Nav (\textbf{ours}) & $0.16 \pm 0.076$ &\checkmark & \checkmark (100$\%$)\\
				\bottomrule    
		\end{tabular}}
	\end{adjustbox}
\end{table}

% \begin{table}[th]
% 	\centering
% 	\caption{Comparison of Local Trajectory planning algorithm computation times.}
% 	\label{tab:ablation_times}
% 	\begin{adjustbox}{width=\linewidth}
% 		{\begin{tabular}{l c c c}
% 				\toprule
    
% 				Algorithm & Times (s) & Smooth & Failure Signal\\
% 				\midrule
    
% 				Line Following & $0.01492 \pm 0.00858$ & \checkmark & \checkmark (58$\%$)\\
    
% 				Splat-Nav (\textbf{ours}) & $0.15241 \pm 0.07588$ &\checkmark & \checkmark (100$\%$)\\
% 				\bottomrule    
% 		\end{tabular}}
% 	\end{adjustbox}
% \end{table}

\section{Recursive Pose Estimation}
Table~\ref{tab:pose_estimation_results_flightroom_larger_error} presents the results in the \textbf{Flightroom} scene with $\delta_R = 50^\circ$ and $\delta_t = \unit[0.2]{m}$. We note that the Gaussian Splatting representation of the Flightroom scene was of much lower quality, which negatively impacted the performance of many of the pose estimation algorithms. As a result, we attempt to mitigate its impact by ensuring that the robot captures informative images during the duration of the problem. 
ICP and Colored-ICP always succeed but yield pose estimates of notably low accuracy, with mean rotation errors of about \unit[120]{deg} and \unit[125]{deg} and translation errors of about \unit[11.59]{m} and \unit[0.73]{m}, respectively. In contrast, \mbox{Splat-Loc-SIFT} fails to produce an estimate in all trials. However, \mbox{Splat-Loc-Glue} achieves a perfect success rate, yields high-accuracy pose estimates with a mean rotation error of about \unit[0.3]{deg} and a mean translation error less than \unit[5]{mm}, and takes an average of \unit[37.74]{ms} per frame. Figure~\ref{fig:pose_estimation_results_flightroom_larger_error_single_run} shows the errors in the pose estimates for a single trial. 

% \begin{table*}[th]
% 	\centering
% 	\caption{Comparison of pose estimation algorithms in the \textbf{Flightroom} scene with $\delta_R = 50^\circ$ and $\delta_t = \unit[0.2]{m}$}
% 	\label{tab:pose_estimation_results_flightroom_larger_error}
% 	\begin{adjustbox}{width=\linewidth}
% 		{\begin{tabular}{l c c c c}
% 				\toprule
% 				Algorithm & Rotation Error (deg.) & Translation Error (m) & Computation Time (secs.) & Success Rate ($\%$) \\
% 				\midrule
% 				ICP \cite{chen1992object} & $1.212 \mathrm{e}^{2} \pm 2.957 \mathrm{e}^{1}$ & $1.159 \mathrm{e}^{1} \pm 2.601 \mathrm{e}^{1}$ & $1.451 \mathrm{e}^{-1} \pm 1.471 \mathrm{e}^{-1}$ & $100$ \\
% 				Colored-ICP \cite{park2017colored} & $1.253 \mathrm{e}^{2} \pm 3.188 \mathrm{e}^{1}$ & $7.354 \mathrm{e}^{-1} \pm 2.540 \mathrm{e}^{-1}$ & $4.847 \mathrm{e}^{-1} \pm 5.472 \mathrm{e}^{-2}$ & $100$ \\
% 				\mbox{Splat-Loc-SIFT} (ours) & $-$ & $-$ & $-$ & $0$ \\
% 				\mbox{Splat-Loc-Glue} (ours) & $\bm{2.539 \mathrm{e}^{-1} \pm 1.543 \mathrm{e}^{-1}}$ & $\bm{3.810 \mathrm{e}^{-3} \pm 2.618 \mathrm{e}^{-3}}$ & $\bm{3.774 \mathrm{e}^{-2} \pm 8.522 \mathrm{e}^{-4}}$ & $100$ \\
% 				\bottomrule
% 		\end{tabular}}
% 	\end{adjustbox}
% \end{table*}

\begin{table*}[th]
	\centering
	\caption{Comparison of pose estimation algorithms in the \textbf{Flightroom} scene with $\delta_R = 50^\circ$ and $\delta_t = \unit[0.2]{m}$}
	\label{tab:pose_estimation_results_flightroom_larger_error}
	\begin{adjustbox}{width=\linewidth}
		{\begin{tabular}{l c c c c}
				\toprule
				Algorithm & Rotation Error (deg.) & Translation Error (m) & Computation Time (secs.) & Success Rate ($\%$) \\
				\midrule
				ICP \cite{chen1992object} & $1.22 \mathrm{e}^{2} \pm 2.96 \mathrm{e}^{1}$ & $1.16 \mathrm{e}^{1} \pm 2.61 \mathrm{e}^{1}$ & $1.46 \mathrm{e}^{-1} \pm 1.48 \mathrm{e}^{-1}$ & $100$ \\
				Colored-ICP \cite{park2017colored} & $1.26 \mathrm{e}^{2} \pm 3.19 \mathrm{e}^{1}$ & $7.36 \mathrm{e}^{-1} \pm 2.54 \mathrm{e}^{-1}$ & $4.85 \mathrm{e}^{-1} \pm 5.48 \mathrm{e}^{-2}$ & $100$ \\
				\mbox{Splat-Loc-SIFT} (ours) & $-$ & $-$ & $-$ & $0$ \\
				\mbox{Splat-Loc-Glue} (ours) & $\bm{2.54 \mathrm{e}^{-1} \pm 1.55 \mathrm{e}^{-1}}$ & $\bm{3.81 \mathrm{e}^{-3} \pm 2.62 \mathrm{e}^{-3}}$ & $\bm{3.78 \mathrm{e}^{-2} \pm 8.53 \mathrm{e}^{-4}}$ & $100$ \\
				\bottomrule
		\end{tabular}}
	\end{adjustbox}
\end{table*}

\begin{figure}[th]
	\centering
	\includegraphics[width=\linewidth, trim={0 7ex 0 12ex}, clip]{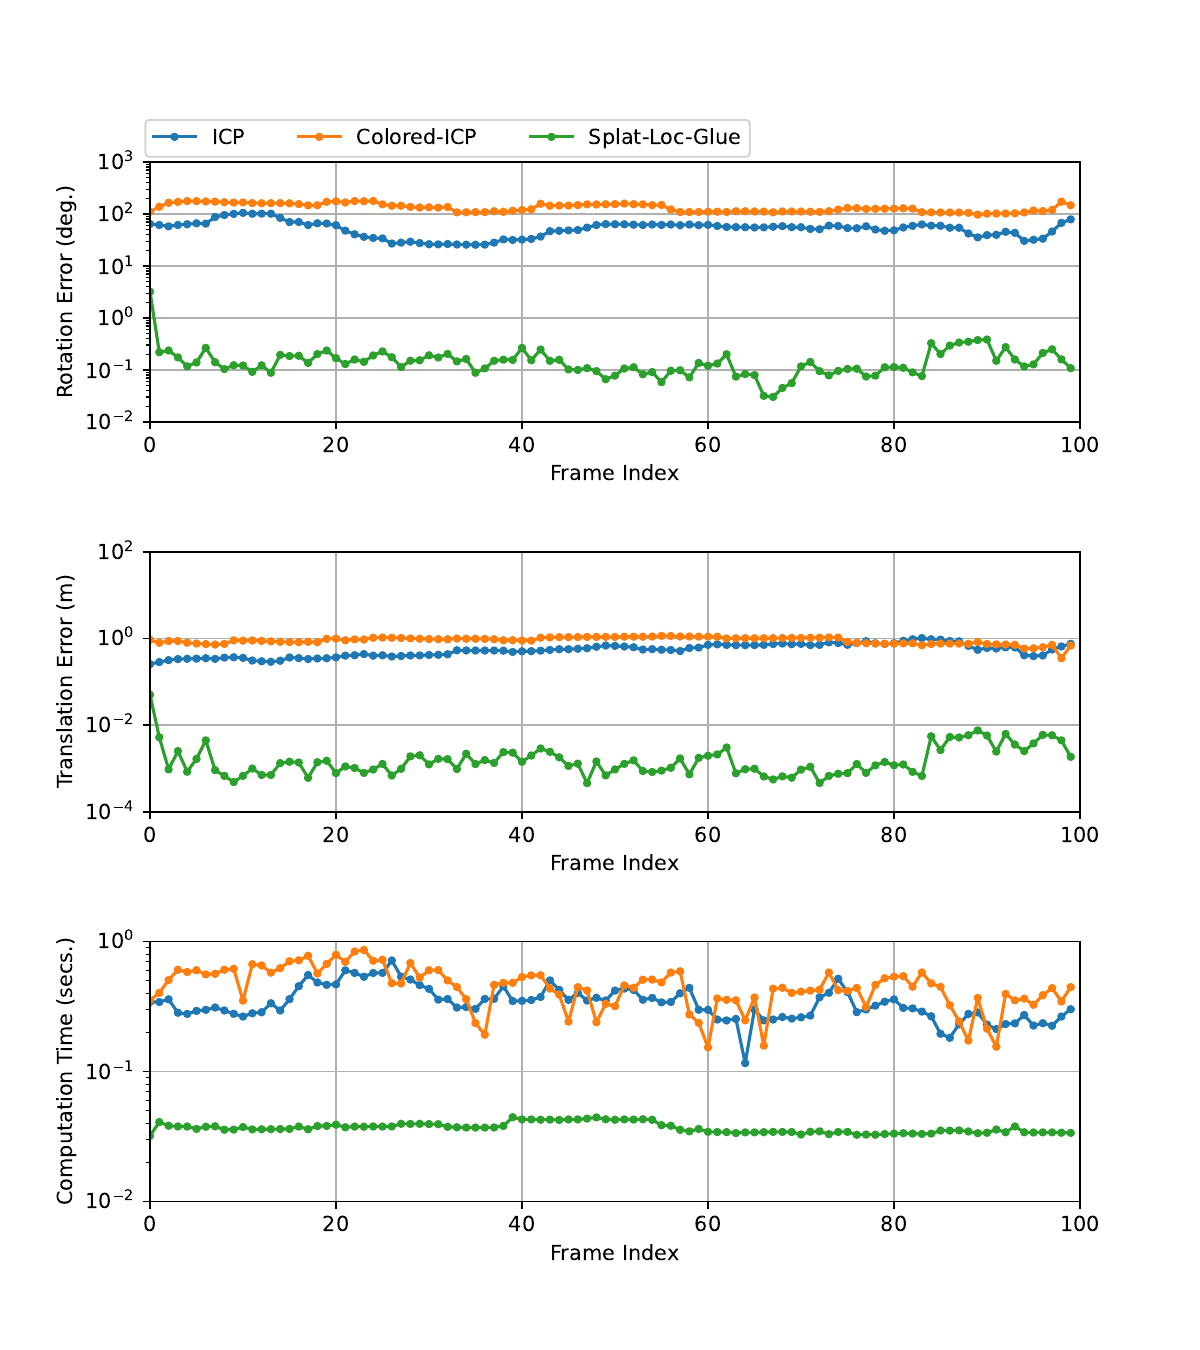}
	\caption{\textbf{Flightroom} Scene with $\delta_R = 50^\circ$ and $\delta_t = \unit[0.2]{m}$---Pose error and computation time per frame achieved by each pose estimation algorithm. \mbox{Splat-Loc-SIFT} was not successful on any trial and is thus omitted in the figure. While ICP and Colored-ICP fail to provide accurate estimates of the robot's pose, \mbox{Splat-Loc-Glue} computes high-accuracy pose estimates.}
    \label{fig:pose_estimation_results_flightroom_larger_error_single_run}
\end{figure}

% \subsection{Pose Estimation: Synthetic Scene}
Here, we examine the performance of each pose estimation algorithm in a synthetic scene \textbf{Stonehenge}, beginning with initial rotation and translation errors of $20$ deg. and $0.1$m. Table~\ref{tab:pose_estimation_results_stonehenge_smaller_error} shows the performance of each algorithm across the ten trials. Similar to the results observed with the real-world scene, \mbox{Splat-Loc-SIFT} and \mbox{Splat-Loc-Glue} yield high-accuracy pose estimates with average rotation and translation errors less than $0.5$ deg and $5$mm respectively, unlike the ICP and Colored-ICP which produce low-accuracy estimates. Moreover, ICP and Colored-ICP seem to diverge in some runs as the estimation procedure proceeds over time, depicted in Figure~\ref{fig:pose_estimation_results_stonehenge_smaller_error_single_run}. In contrast, \mbox{Splat-Loc-Glue} achieves a perfect success rate, in contrast with \mbox{Splat-Loc-SIFT}, which achieves a $90\%$ success rate, in addition to attaining the fastest computation time.

% \begin{table*}[th]
% 	\centering
% 	\caption{Comparison of pose estimation algorithms in the \textbf{Stonehenge} scene with $\delta_R = 20^\circ$ and $\delta_t = \unit[0.1]{m}$.
%  % across $10$ trials.
%         }
% 	\label{tab:pose_estimation_results_stonehenge_smaller_error}
% 	\begin{adjustbox}{width=\linewidth}
% 		{\begin{tabular}{l c c c c}
% 				\toprule
% 				Algorithm & Rotation Error (deg.) & Translation Error (m) & Computation Time (secs.) & Success Rate ($\%$) \\
% 				\midrule
% 				ICP \cite{chen1992object} & $9.702 \mathrm{e}^{1} \pm 3.006 \mathrm{e}^{1}$ & $1.085 \mathrm{e}^{0} \pm 7.958 \mathrm{e}^{-1}$ & $3.604 \mathrm{e}^{-1} \pm 5.036 \mathrm{e}^{-2}$ & $100$ \\
% 				Colored-ICP \cite{park2017colored} & $7.185 \mathrm{e}^{1} \pm 3.224 \mathrm{e}^{1}$ & $5.175 \mathrm{e}^{-1} \pm 2.162 \mathrm{e}^{-1}$ & $3.678 \mathrm{e}^{-1} \pm 6.378 \mathrm{e}^{-2}$ & $100$ \\
% 				\mbox{Splat-Loc-SIFT} (ours) & $1.962 \mathrm{e}^{-1} \pm 2.690 \mathrm{e}^{-2}$ & $3.033 \mathrm{e}^{-3} \pm 4.268 \mathrm{e}^{-4}$ & $1.399 \mathrm{e}^{-1} \pm 5.727 \mathrm{e}^{-3}$ & $90$ \\
% 				\mbox{Splat-Loc-Glue} (ours) & $\bm{2.114 \mathrm{e}^{-1} \pm 2.265 \mathrm{e}^{-1}}$ & $\bm{2.962 \mathrm{e}^{-3} \pm 2.420 \mathrm{e}^{-3}}$ & $\bm{4.554 \mathrm{e}^{-2} \pm 1.119 \mathrm{e}^{-3}}$ & $100$ \\
% 				\bottomrule
% 		\end{tabular}}
% 	\end{adjustbox}
% \end{table*}

\begin{table*}[th]
	\centering
	\caption{Comparison of pose estimation algorithms in the \textbf{Stonehenge} scene with $\delta_R = 20^\circ$ and $\delta_t = \unit[0.1]{m}$.
 % across $10$ trials.
        }
	\label{tab:pose_estimation_results_stonehenge_smaller_error}
	\begin{adjustbox}{width=\linewidth}
		{\begin{tabular}{l c c c c}
				\toprule
				Algorithm & Rotation Error (deg.) & Translation Error (m) & Computation Time (secs.) & Success Rate ($\%$) \\
				\midrule
				ICP \cite{chen1992object} & $9.71 \mathrm{e}^{1} \pm 3.01 \mathrm{e}^{1}$ & $1.09 \mathrm{e}^{0} \pm 7.96 \mathrm{e}^{-1}$ & $3.61 \mathrm{e}^{-1} \pm 5.04 \mathrm{e}^{-2}$ & $100$ \\
				Colored-ICP \cite{park2017colored} & $7.19 \mathrm{e}^{1} \pm 3.23 \mathrm{e}^{1}$ & $5.18 \mathrm{e}^{-1} \pm 2.17 \mathrm{e}^{-1}$ & $3.68 \mathrm{e}^{-1} \pm 6.38 \mathrm{e}^{-2}$ & $100$ \\
				\mbox{Splat-Loc-SIFT} (ours) & $1.97 \mathrm{e}^{-1} \pm 2.69 \mathrm{e}^{-2}$ & $3.04 \mathrm{e}^{-3} \pm 4.27 \mathrm{e}^{-4}$ & $1.40 \mathrm{e}^{-1} \pm 5.73 \mathrm{e}^{-3}$ & $90$ \\
				\mbox{Splat-Loc-Glue} (ours) & $\bm{2.12 \mathrm{e}^{-1} \pm 2.27 \mathrm{e}^{-1}}$ & $\bm{2.97 \mathrm{e}^{-3} \pm 2.42 \mathrm{e}^{-3}}$ & $\bm{4.56 \mathrm{e}^{-2} \pm 1.12 \mathrm{e}^{-3}}$ & $100$ \\
				\bottomrule
		\end{tabular}}
	\end{adjustbox}
\end{table*}

\begin{figure}[th]
	\centering
	\includegraphics[width=\linewidth, trim={0 7ex 0 12ex}, clip]{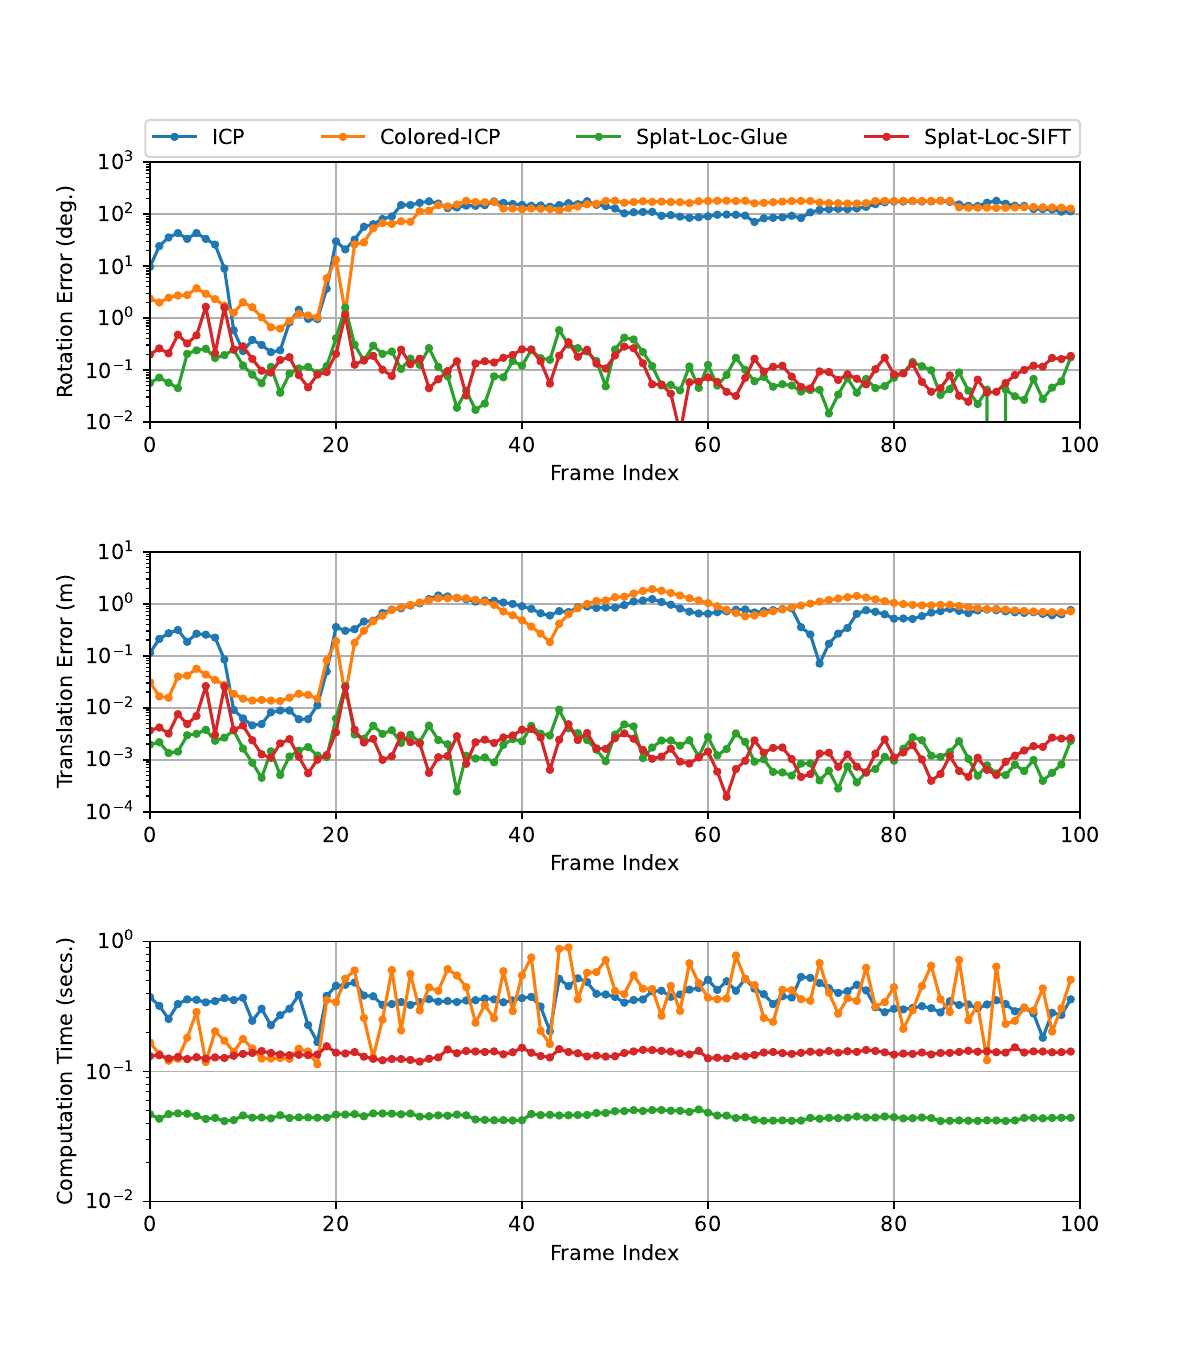}
	\caption{\textbf{Stonehenge} Scene with $\delta_R = 20^\circ$ and $\delta_t = \unit[0.1]{m}$---While ICP and Colored-ICP diverge over time, \mbox{Splat-Loc-SIFT} and \mbox{Splat-Loc-Glue} do not diverge, producing high-accuracy estimates.}
	\label{fig:pose_estimation_results_stonehenge_smaller_error_single_run}
\end{figure}

In addition, we examine the performance of the pose estimation algorithmsin problems with a larger error in the initial estimate of the pose, with $\delta_R = 30^\circ$ and $\delta_t = \unit[0.5]{m}$. We present the performance of each algorithm on each metric in Table~\ref{tab:pose_estimation_results_stonehenge_larger_error}, where we note that ICP and Colored-ICP do not provide accurate estimate of the robot's pose. Moreover, the pose estimation errors achieved by ICP and Colored-ICP have a significant variance. In contrast, \mbox{Splat-Loc-SIFT} and \mbox{Splat-Loc-Glue} yield pose estimates of high accuracy with average rotation and translation errors less than $0.5$ deg. and $5$mm, respectively, similar to the setting with low errors in the initial pose estimate. However, \mbox{Splat-Loc-SIFT} achieves a lower success rate, compared to \mbox{Splat-Loc-Glue}, which achieves a perfect success rate. In Figure~\ref{fig:pose_estimation_results_stonehenge_larger_error_single_run}, we show the estimation errors for a single run, highlighting the high variance in the errors associated with the pose estimates computed Colored-ICP. ICP fails to yield a pose estimate of relatively high accuracy for the duration of the problem.

\begin{table*}[th]
	\centering
	\caption{Comparison of pose estimation algorithms in the \textbf{Stonehenge} scene with $\delta_R = 30^\circ$ and $\delta_t = \unit[0.5]{m}$.
 % across $10$ trials.
        }
	\label{tab:pose_estimation_results_stonehenge_larger_error}
	\begin{adjustbox}{width=\linewidth}
		{\begin{tabular}{l c c c c}
				\toprule
				Algorithm & Rotation Error (deg.) & Translation Error (m) & Computation Time (secs.) & Success Rate ($\%$) \\
				\midrule
				ICP \cite{chen1992object} & $1.31 \mathrm{e}^{2} \pm 2.26 \mathrm{e}^{1}$ & $3.70 \mathrm{e}^{0} \pm 5.54 \mathrm{e}^{0}$ & $1.22 \mathrm{e}^{-1} \pm 1.53 \mathrm{e}^{-1}$ & $100$ \\
				Colored-ICP \cite{park2017colored} & $9.49 \mathrm{e}^{1} \pm 5.13 \mathrm{e}^{1}$ & $5.74 \mathrm{e}^{-1} \pm 2.88 \mathrm{e}^{-1}$ & $4.88 \mathrm{e}^{-1} \pm 1.04 \mathrm{e}^{-1}$ & $20$ \\
				\mbox{Splat-Loc-SIFT} (ours) & $\bm{2.17 \mathrm{e}^{-1} \pm 3.69 \mathrm{e}^{-2}}$ & $3.34 \mathrm{e}^{-3} \pm 5.63 \mathrm{e}^{-4}$ & $1.39 \mathrm{e}^{-1} \pm 3.15 \mathrm{e}^{-3}$ & $70$ \\
				\mbox{Splat-Loc-Glue} (ours) & $2.20 \mathrm{e}^{-1} \pm 2.03 \mathrm{e}^{-1}$ & $\bm{3.15 \mathrm{e}^{-3} \pm 2.10 \mathrm{e}^{-3}}$ & $\bm{4.51 \mathrm{e}^{-2} \pm 6.11 \mathrm{e}^{-4}}$ & $100$ \\
				\bottomrule
		\end{tabular}}
	\end{adjustbox}
\end{table*}

% \begin{table*}[th]
% 	\centering
% 	\caption{Comparison of pose estimation algorithms in the \textbf{Stonehenge} scene with $\delta_R = 30^\circ$ and $\delta_t = \unit[0.5]{m}$.
%  % across $10$ trials.
%         }
% 	\label{tab:pose_estimation_results_stonehenge_larger_error}
% 	\begin{adjustbox}{width=\linewidth}
% 		{\begin{tabular}{l c c c c}
% 				\toprule
% 				Algorithm & Rotation Error (deg.) & Translation Error (m) & Computation Time (secs.) & Success Rate ($\%$) \\
% 				\midrule
% 				ICP \cite{chen1992object} & $1.303 \mathrm{e}^{2} \pm 2.254 \mathrm{e}^{1}$ & $3.697 \mathrm{e}^{0} \pm 5.533 \mathrm{e}^{0}$ & $1.217 \mathrm{e}^{-1} \pm 1.527 \mathrm{e}^{-1}$ & $100$ \\
% 				Colored-ICP \cite{park2017colored} & $9.489 \mathrm{e}^{1} \pm 5.128 \mathrm{e}^{1}$ & $5.737 \mathrm{e}^{-1} \pm 2.880 \mathrm{e}^{-1}$ & $4.879 \mathrm{e}^{-1} \pm 1.038 \mathrm{e}^{-1}$ & $20$ \\
% 				\mbox{Splat-Loc-SIFT} (ours) & $\bm{2.164 \mathrm{e}^{-1} \pm 3.682 \mathrm{e}^{-2}}$ & $3.335 \mathrm{e}^{-3} \pm 5.628 \mathrm{e}^{-4}$ & $1.384 \mathrm{e}^{-1} \pm 3.145 \mathrm{e}^{-3}$ & $70$ \\
% 				\mbox{Splat-Loc-Glue} (ours) & $2.193 \mathrm{e}^{-1} \pm 2.024 \mathrm{e}^{-1}$ & $\bm{3.141 \mathrm{e}^{-3} \pm 2.099 \mathrm{e}^{-3}}$ & $\bm{4.507 \mathrm{e}^{-2} \pm 6.105 \mathrm{e}^{-4}}$ & $100$ \\
% 				\bottomrule
% 		\end{tabular}}
% 	\end{adjustbox}
% \end{table*}

\begin{figure}[th]
	\centering
	\includegraphics[width=\linewidth, trim={0 7ex 0 12ex}, clip]{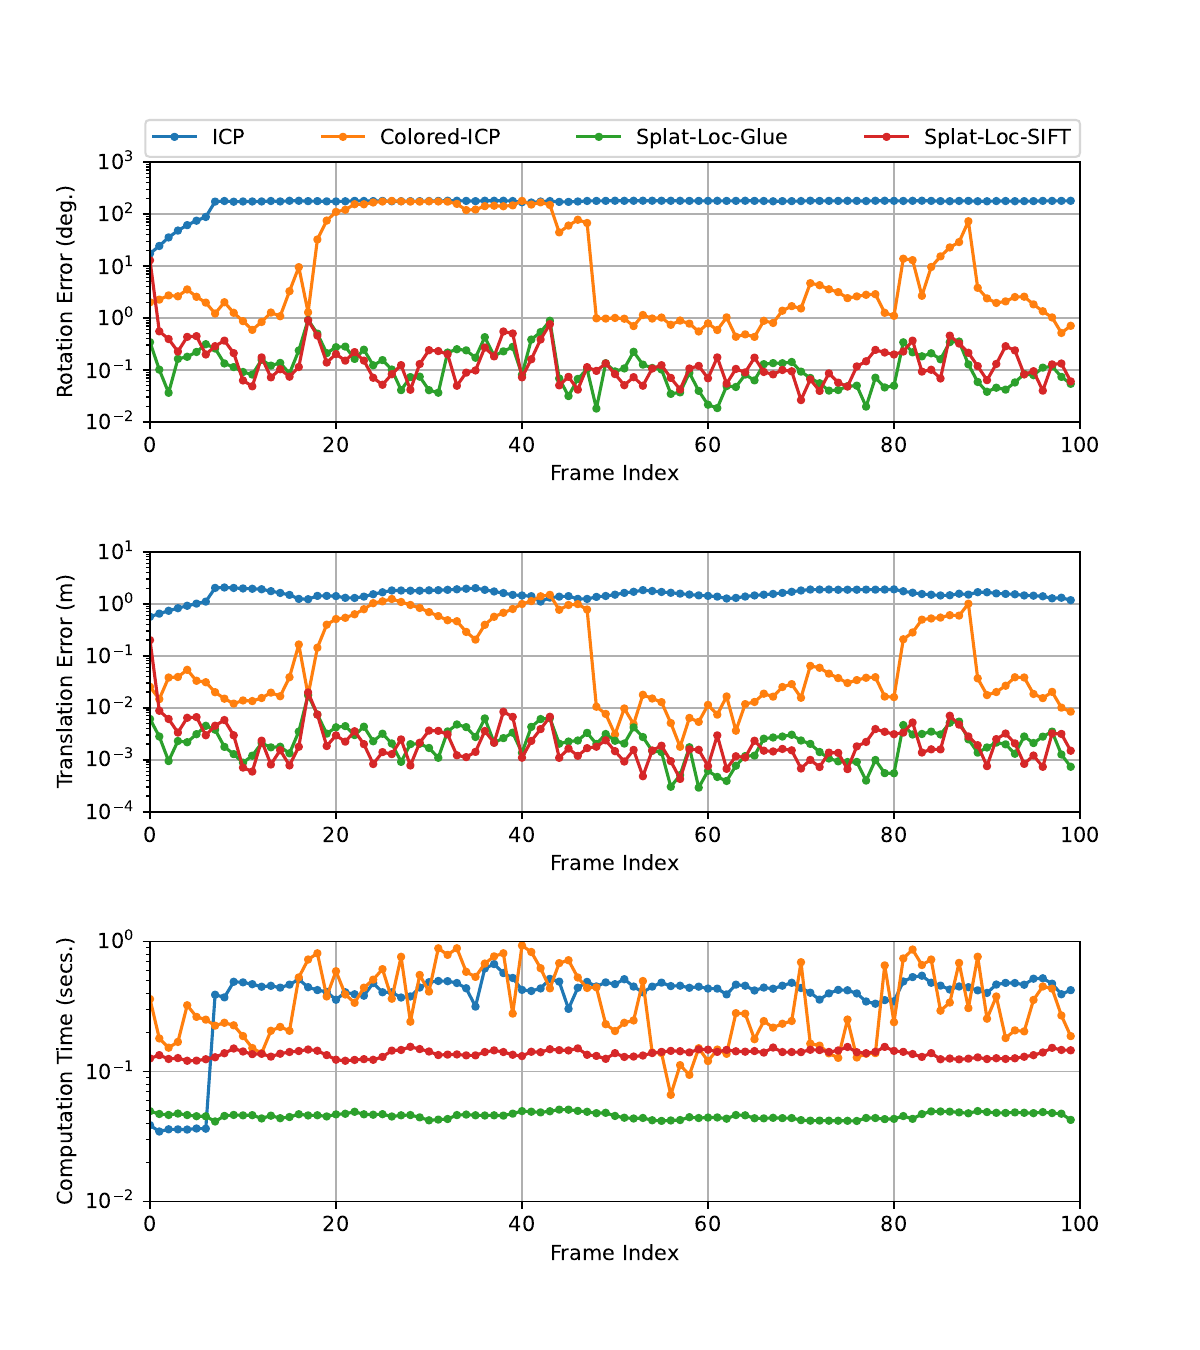}
	\caption{Stonehenge Scenewith $\delta_R = 30^\circ$ and $\delta_t = \unit[0.5]{m}$---\mbox{Splat-Loc-SIFT} and \mbox{Splat-Loc-Glue} produce pose estimates of the highest accuracy, compared to ICP and Colored-ICP. Further, \mbox{Splat-Loc-Glue} requires the least computation time per frame.}
	\label{fig:pose_estimation_results_stonehenge_larger_error_single_run}
\end{figure}
